# Supplementary material for: Map-Aware Human Pose Prediction for Robot Follow-Ahead
Source: arXiv:2403.13294 source file (2024-03-20)
Supplement: Supplementary file 1 [file qualitative.tex]

\begin{figure}[htp]
    \centering
    \includegraphics[width=1.0\columnwidth]{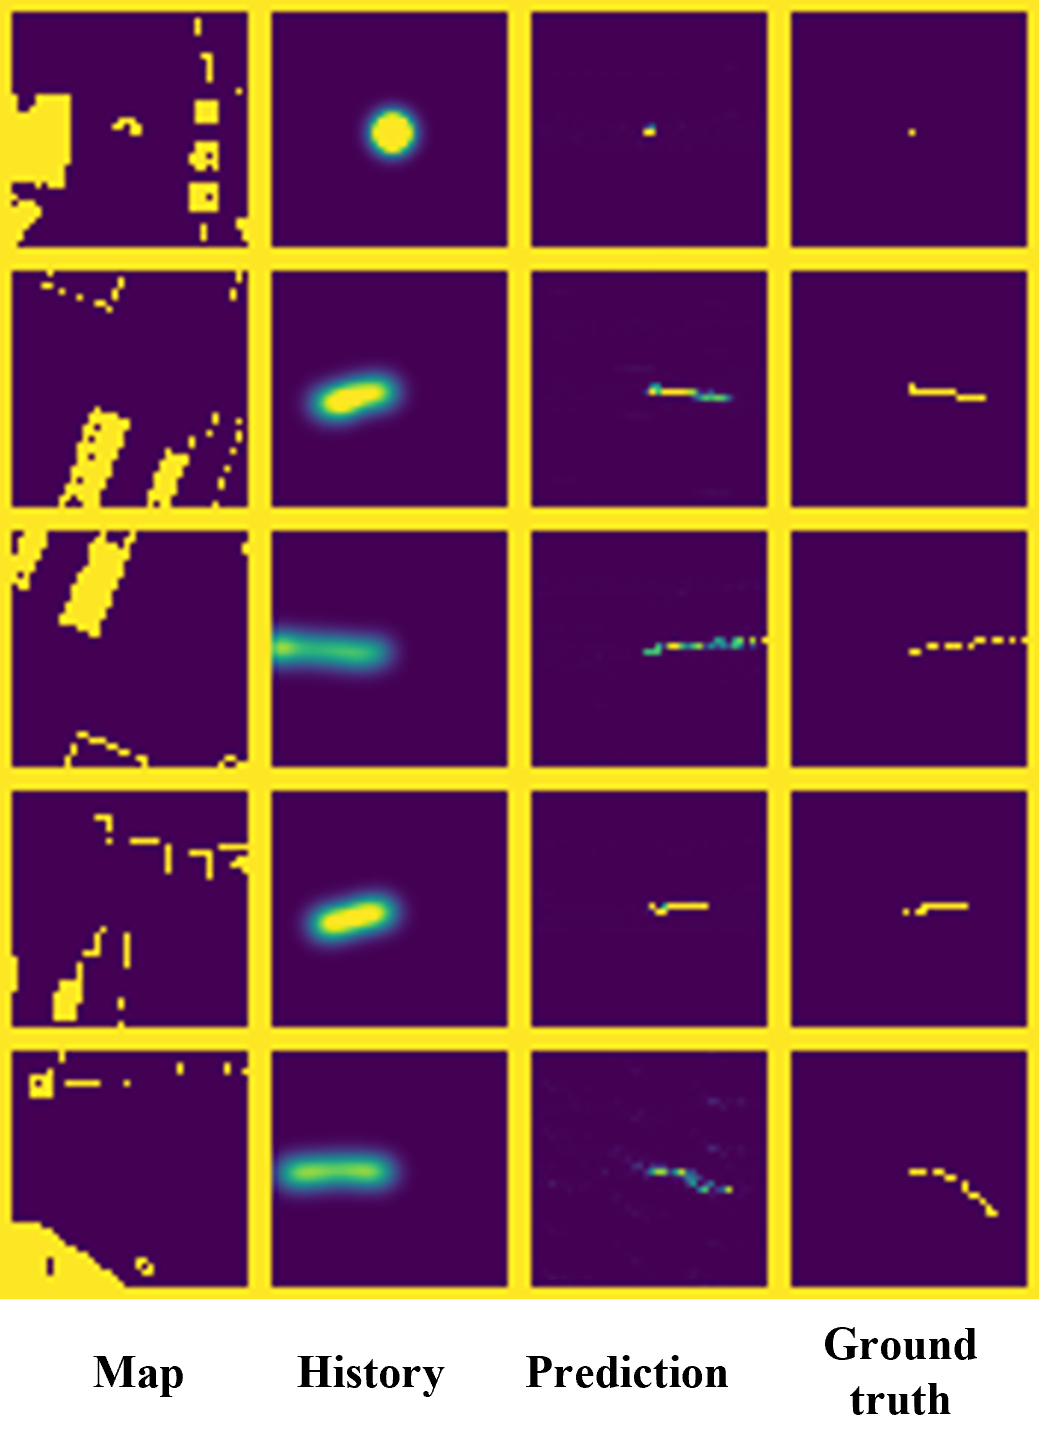}
    \caption{\textbf{Path prediction}. Each row is a sample case. From the left to the right column, we show the local occupancy map, human trajectory map history, human trajectory map prediction, and human trajectory map ground truth respectively.}
    \label{fig: path}
\end{figure}

We show more qualitative results in this section. In Fig.~\ref{fig: path}, we show the human path prediction from our Pathnet conditioned on the local map. Each cell is either a local occupancy map (first column) or a trajectory map. The map is drawn in the latest actor's frame $\mathbf{X}_{N}$. The origin point (the latest actor's position) is located at the center of the figure. $X$ and $Y$ axes in the actor frame are aligned with the image coordinate axes. Therefore, for example, in the occupancy map, the actor is standing in the middle of the map, heading towards to right direction ($x$-axis) of the map. In the trajectory map, the actor comes from the left part and heads to the right part.

The first column shows the occupancy local map we use. Environments that the human would avoid are labeled as 1, and open space as 0. The second column shows the past trajectory of the human. We use the Gaussian distribution heatmap as the input to the network. The third column shows the predicted trajectory map, and the fourth shows the ground truth. As shown in Fig.~\ref{fig: path}, conditioned on the local occupancy map (first column) and the past trajectory map (second column), we predict the future trajectory map (third column) which should be similar to the ground truth (fourth column).
